# Supplementary material for: Symmetric Rank-One Quasi-Newton Methods for Deep Learning Using Cubic Regularization
Source: arXiv:2502.12298 source file (2025-02-17)
Supplement: Supplementary file 3 [file AppendixResults.tex]

The ARCs-LSR1 method requires some history from the past to form the Limited-memory SR1 approximation. The history stores a set of steps `$\mathbf{s}$' and their corresponding change in gradients `$\mathbf{y}$'. This is the most important parameter for the proposed approach - as the number of history pairs increase, the approximation begins converging to the true Hessian. However, we cannot have a full-rank approximation, so the number of history pairs are limited. In addition, in the context of deep learning, a high memory parameter might not be beneficial.

To empirically show this, we run a set of experiments by varying the batch-size and the the number of iterations for each batch and present results on the MNIST classification task. We selected a history-size of $5, 10, 15, 29, 50$ and $100$.

\begin{table}[!htb]
    \begin{tabular}{cc}
        \subfloat[]{\adjincludegraphics[width=0.45\linewidth, trim={{.02\width}  0 {.03\width} {0.15\height}}, clip]{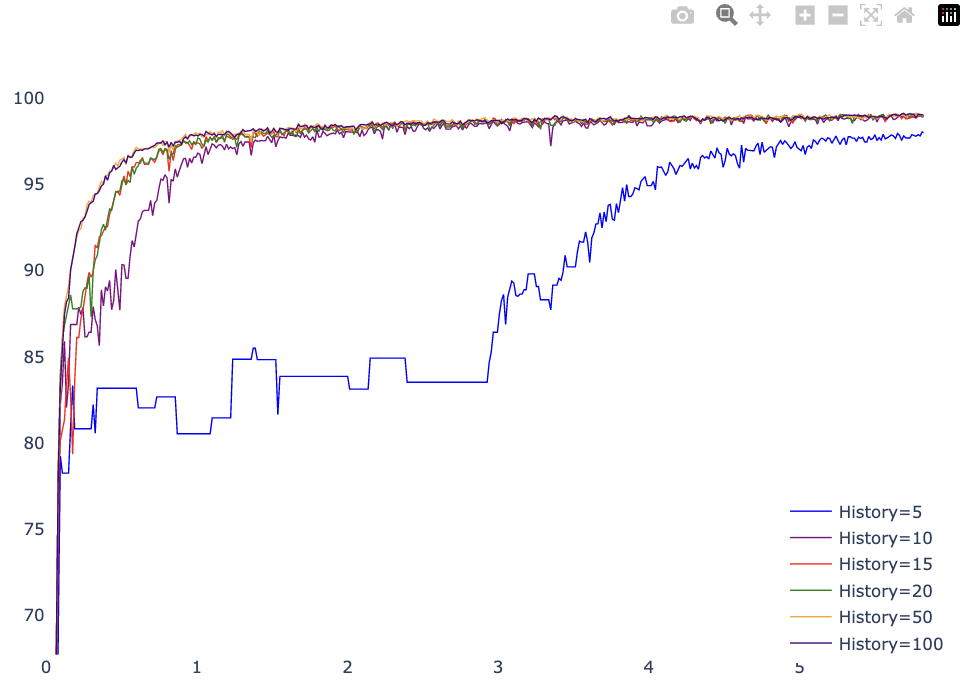}} 
        & 
        \subfloat[]{\adjincludegraphics[width=0.45\linewidth,trim={{.05\width}  0 {.03\width} {0.11\height}}, clip]{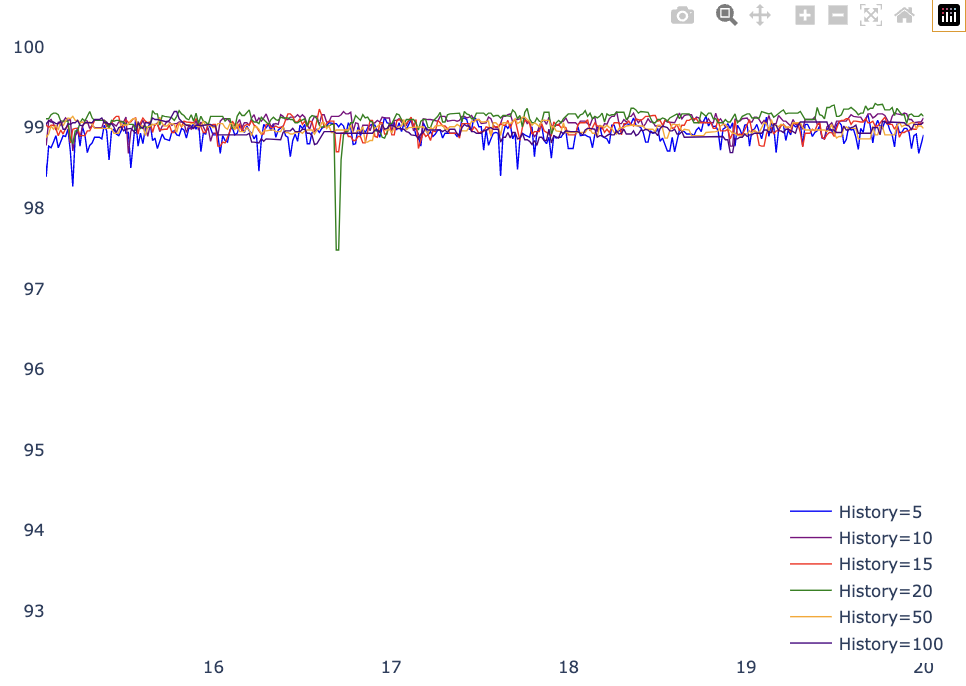}}
        \\
        \subfloat[]{\adjincludegraphics[width=0.45\linewidth, trim={{.02\width}  0 {.03\width} {0.05\height}}, clip]{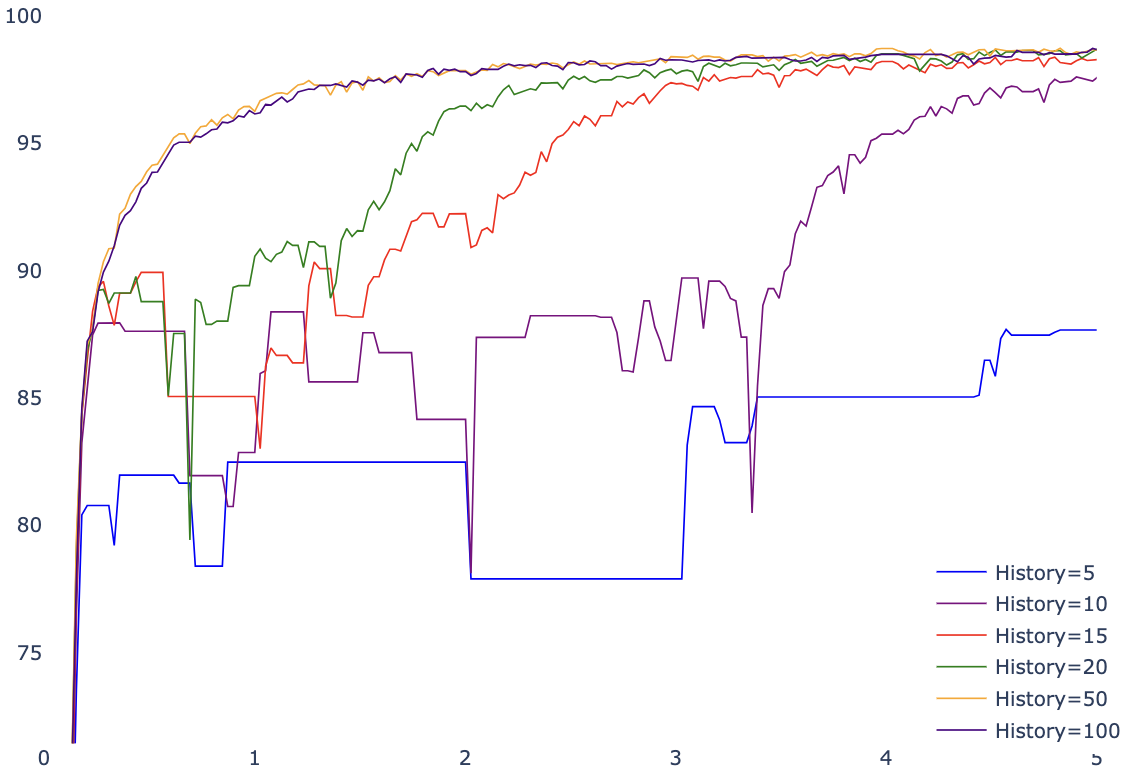}} 
        & 
        \subfloat[]{\adjincludegraphics[width=0.45\linewidth,trim={{.05\width}  0 {.03\width} {0\height}}, clip]{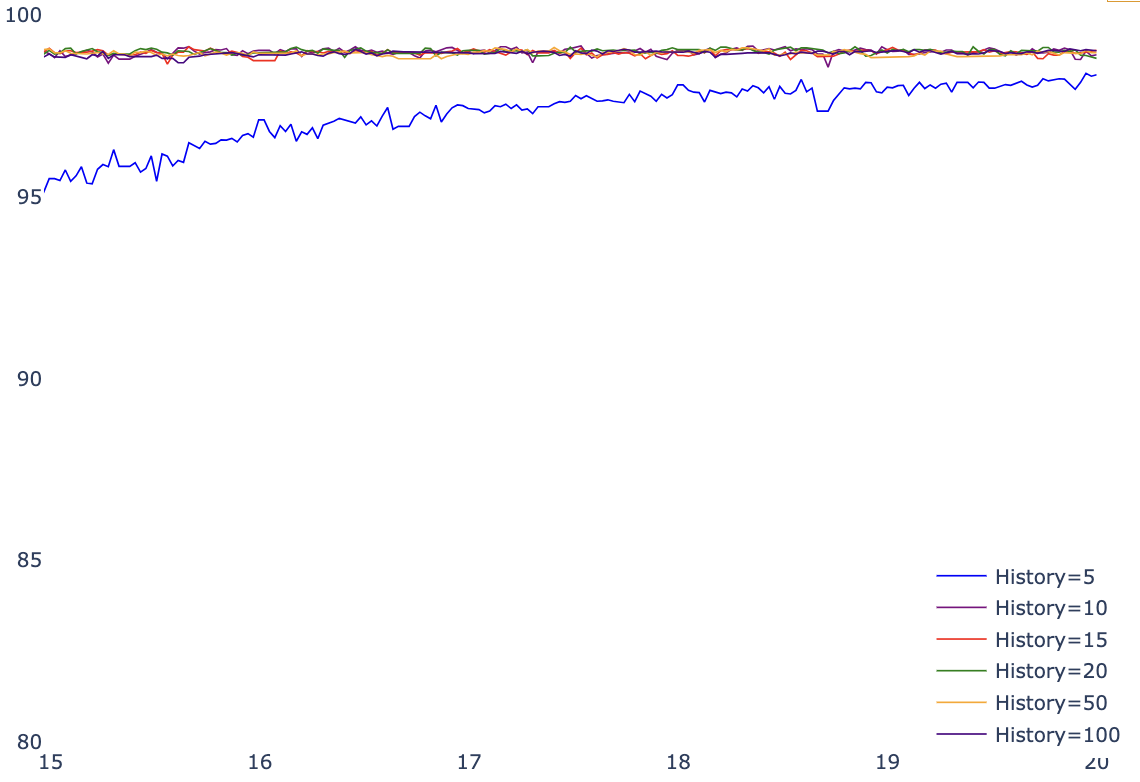}}
        \\
        \subfloat[]{\adjincludegraphics[width=0.45\linewidth, trim={{.02\width}  0 {.03\width} {0\height}}, clip]{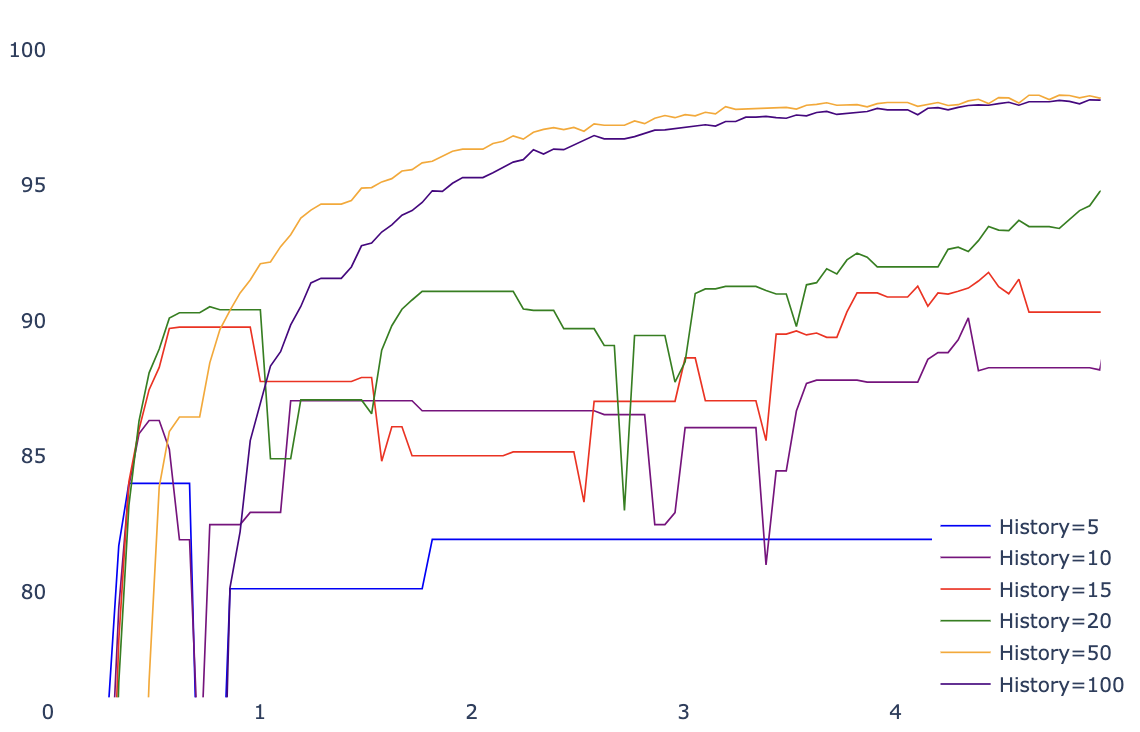}} 
        & 
        \subfloat[]{\adjincludegraphics[width=0.45\linewidth,trim={{.05\width}  0 {.03\width} {0.11\height}}, clip]{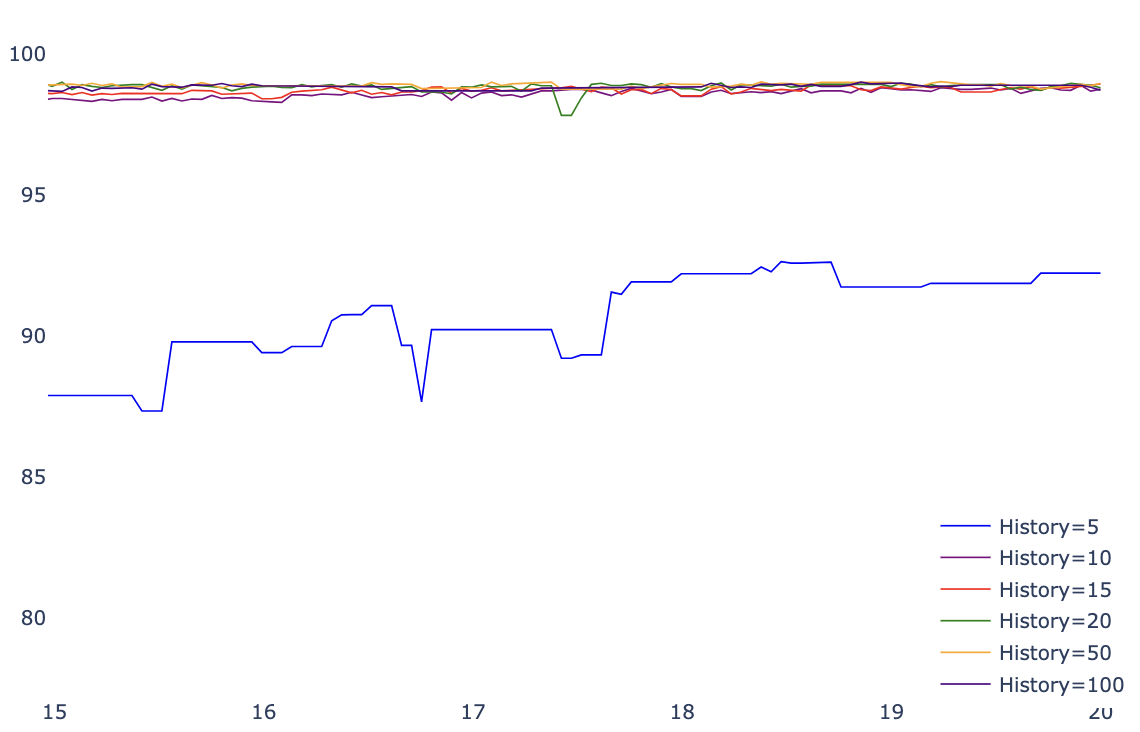}}
        \\
        \subfloat[]{\adjincludegraphics[width=0.45\linewidth, trim={{.02\width}  0 {.03\width} {0\height}}, clip]{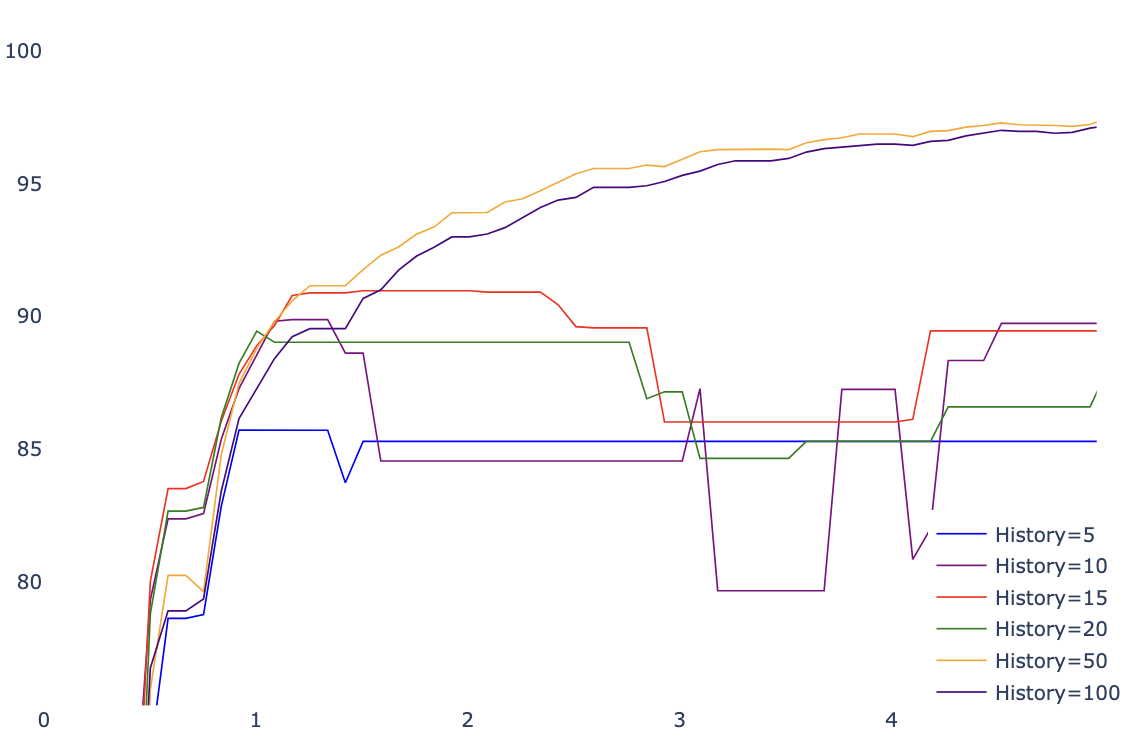}} 
        &
        \subfloat[]{\adjincludegraphics[width=0.45\linewidth,trim={{.05\width}  0 {.03\width} {0.11\height}}, clip]{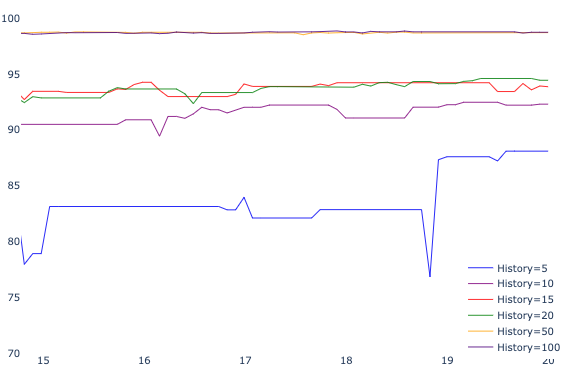}}
    \end{tabular}
    \caption{\textbf{MNIST Classification:} We choose from different batch-sizes of $[128, 256, 512]$ and $1024$. Maximum-iterations per-batch is fixed to $1$. The left-column [(a), (c) and (d)] represent the early epochs [1-5] while the second column [b, d and f] represent the late epochs [15-20]. Row 1 presents the results with a batch-size of 128, Row 2 presents the results with a batch-size of 256, Row 3 - batch-size of 512 and Row 4 - batch-size of 1024.}\label{fig:appnd:batch-sizes}
\end{table}

\begin{table}
    
    \begin{tabular}{cc}
         \subfloat[]{\adjincludegraphics[width=0.45\linewidth, trim={{.02\width}  0 {.03\width} {0\height}}, clip]{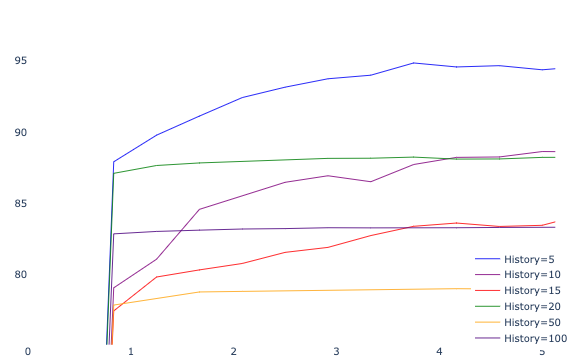}} \hspace{5mm} 
         & 
         \subfloat[]{\adjincludegraphics[width=0.45\linewidth,trim={{.05\width}  0 {.03\width} {0.11\height}}, clip]{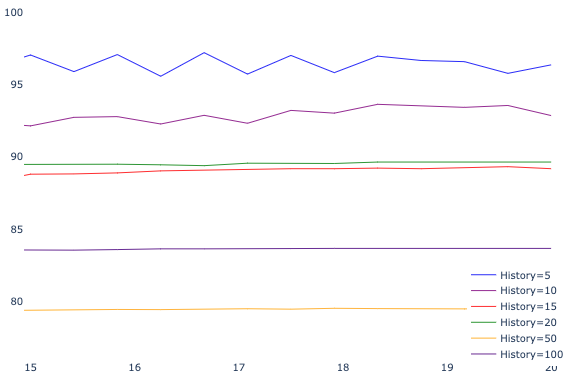}}  
         \\
         \subfloat[]{\adjincludegraphics[width=0.45\linewidth, trim={{.02\width}  0 {.03\width} {0\height}}, clip]{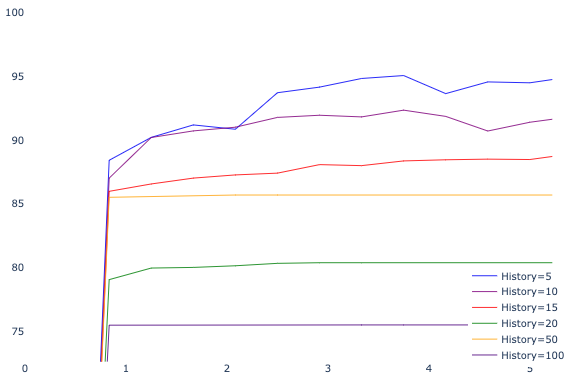}} 
         & 
         \subfloat[]{\adjincludegraphics[width=0.45\linewidth,trim={{.05\width}  0 {.03\width} {0.05\height}}, clip]{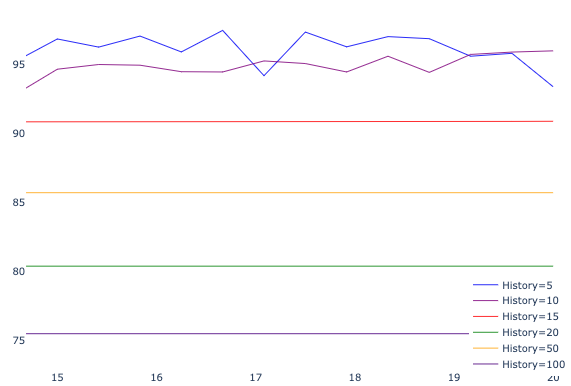}}
         \\
         \subfloat[]{\adjincludegraphics[width=0.45\linewidth, trim={{.02\width}  0 {.03\width} {0\height}}, clip]{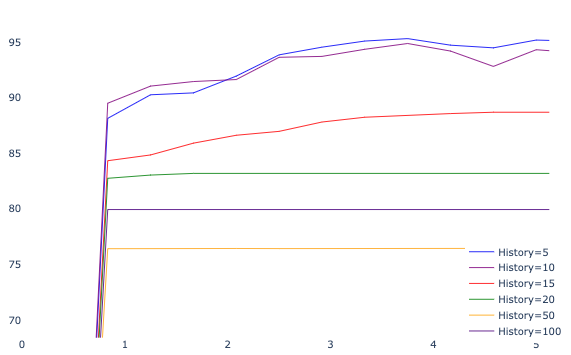}} 
         & 
         \subfloat[]{\adjincludegraphics[width=0.45\linewidth,trim={{.05\width}  0 {.03\width} {0.05\height}}, clip]{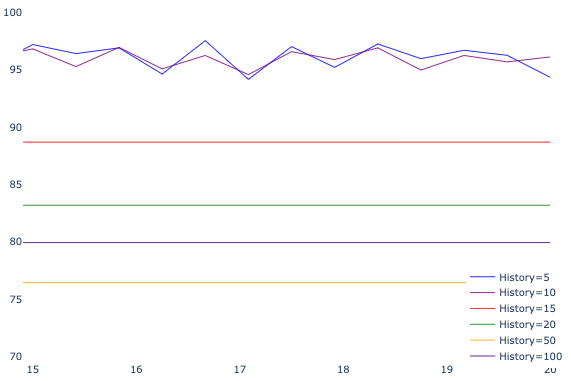}}
    \end{tabular}
    \caption{\textbf{MNIST classification:} The figure shows the classification response for different max-iterations $[10, 15, 20]$ with a history-size of size of $[5, 10, 14, 20, 50 \text{ and } 100]$.  The batch-size is fixed to $128$ images. The left-column [(a), (c) and (e)] present the early epochs $[1-5]$ while the second column [(b), (d) and (f)] present the late epochs $[15-20]$. Row $1$ presents the results with a max-iterations of $10$, Row $2$ presents the results with a max-iterations of $15$ and Row 3 presents the results with max-iterations of $20$.}\label{fig:appnd:Max-iterations}
\end{table}

% \begin{figure}[!htb]
%     \centering
    
%     \label{appnd:fig:max-iters-20}
% \end{figure}

\subsection{Different max-iterations}
\label{appnd:subsec:Diffiters}
The max-iterations determines how many times the proposed approach is applied to each individual batch for an optimization step and its corresponding history update ($\mathbf{s}, \mathbf{y}$). For the most ideal condition, we consider the trade-off between computational complexity and improvement of accuracy. This means the accuracy of prediction does not increase significantly with the increase in the upper bound of iterations. We fix the batch-size to $128$ and switch the batch-size between a batch-size of $10, 15$ and $20$.

The results are presented in Fig.\ \ref{fig:appnd:Max-iterations}. From these results, it was certain that a maximum iteration of 10 was ideal. 

\subsection{Different batch-sizes}
\label{appnd:batch-sizes}
For this experiment, we chose from batch-sizes of $128, 256, 512$ and $1024$. We fixed the maximum-iterations to $1$. The results are presented in Fig.\ \ref{fig:appnd:batch-sizes}.
