# Supplementary material for: Symmetric Rank-One Quasi-Newton Methods for Deep Learning Using Cubic Regularization
Source: arXiv:2502.12298 source file (2025-02-17)
Supplement: Supplementary file 6 [file DiffHistSizes.tex]

\begin{figure}[!ht]
    \centering
    \subfloat[All epochs]{\adjincludegraphics[width=0.45\linewidth]{Figures/Appendix/Appendix-batch-size-128-max-iters-1-hist-all-epochs-all.png}\label{Fig:Appnd:diffhistsizesall}}\hfill
    \subfloat[Early epochs]{\adjincludegraphics[width=0.45\linewidth]{Figures/Appendix/Appendix-batch-size-128-max-iters-1-hist-all-epochs-early.png}\label{Fig:Appnd:diffhistsizesearly}}\\
    \par
    \subfloat[Late epochs]{\adjincludegraphics[width=0.45\linewidth]{Figures/Appendix/Appendix-batch-size-128-max-iters-1-hist-all-epochs-late.png}\label{Fig:Appnd:diffhistsizeslate}}
    \caption{We present the results for different history sizes of {5, 10, 15, 20. 50, 100}. We choose the no. of iterations to be 1 for each experiment.}\label{Fig:Append:diffhist}
\end{figure}

The results for different history sizes is present in figure \ref{Fig:Append:diffhist}.

% \adjincludegraphics[width=\linewidth]{Figures/Appendix/Appendix-batch-size-128-max-iters-1-hist-all-epochs-late.png}\label{Appnd:diffhistsizes}
